# Supplementary material for: A New Journey from SDRTV to HDRTV
Source: arXiv:2108.07978 source file (2021-09-25)
Supplement: Supplementary file 1 [file supp.pdf]

# A New Journey from SDRTV to HDRTV
# Supplementary Material

Xiangyu Chen[1*] Zhengwen Zhang[1*] Jimmy S. Ren[2,3] Lynhoo Tian[2] Yu Qiao[1,4] Chao Dong[1†]
[1]ShenZhen Key Lab of Computer Vision and Pattern Recognition, SIAT-SenseTime Joint Lab,
Shenzhen Institute of Advanced Technology, Chinese Academy of Sciences [2]SenseTime Research
[3]Qing Yuan Research Institute, Shanghai Jiao Tong University [4]Shanghai AI Laboratory, Shanghai
{chxy95, zhengwen.zhang02, jimmy.sj.ren, lynhoo.tian}@gmail.com {yu.qiao, chao.dong}@siat.ac.cn

## 1. Overview

In this supplementary material, we present additional explanations and analyses to complement the main manuscript. First, we provide more details about the formation pipeline include the principle to simplify the pipeline and the specific explanations of diagrams and curves in the pipeline. Second, we introduce the implementation details for training our networks. Third, we present additional quantitative and qualitative analyses of our method. Fourth, we provide more additional explanations about visualization and the user study. Finally, we demonstrate the performance of our method in realistic scenes.

## 2. More details about the formation pipeline

In this section, we aim at providing more details about the formation pipeline in two aspects: (1) The principle to simplify the formation pipeline. (2) Specific explanations of the diagrams and curves.

### 2.1. The principle to simplify the formation pipeline

In [10], the LDR image formation pipeline is simplified as in Fig. 1(a). The pipeline contains three main parts in the camera pipeline for HDR-to-LDR, which are dynamic range clipping, non-linear mapping (i.e., applying transfer function in the paper) and quantization. In this pipeline, "HDR" represents the scene radiance and color mapping is not involved. Similar to this pipeline, for SDRTV/HDRTV formation, the process also contains dynamic range compression, applying transfer function and quantization. However, there are two essential differences between the LDR formation pipeline and SDRTV/HDRTV pipeline. First, for LDR-to-HDR, the LDR image is generated from HDR scene radiance, thus LDR-to-HDR is a kind of reverse process to some extent. In contrast, SDRTV and HDRTV are generated from the same raw data (or resource in Log format) by different operations for different standards as in Fig. 1(b). From this perspective, SDRTV-to-HDRTV is more like an image-to-image translation task. Second, color conversion is generally not involved in LDR-to-HDR, as the "HDR" has been converted from camera RGB to sRGB, which is generally encoded in the same color gamut as LDR by default. However, gamut expansion is a crucial step in SDRTV-to-HDRTV. Therefore, we add gamut mapping in SDRTV/HDRTV formation pipeline. Overall, we provide the formation pipeline to illustrate the key steps in production leading to the difference between SDRTV and HDRTV content.

### 2.2. Specific explanations of the diagrams and curves

In the main paper, we provide sketch maps of four operations for leading viewers to focus on the formation pipeline and corresponding solution pipeline. In this subsection, we take specific explanations of the diagrams and curves.

**Tone mapping**. We draw the diagram and curve of the tone mapping operation by using Hable tone mapping [2] shown in Fig. 2, which can be formulated as:

$$T_{Hable} = f_{Hable}(I) = h(1.6 * k * I)/h(w) \quad (1)$$

*indicates contribute equally. †Corresponding author.

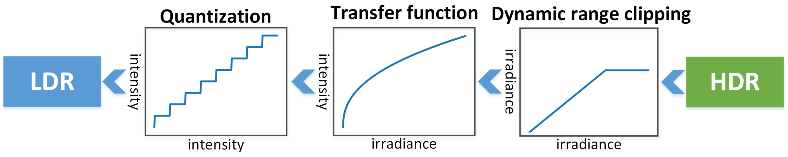

(a) LDR imgae formation pipeline in SingleHDR [10]

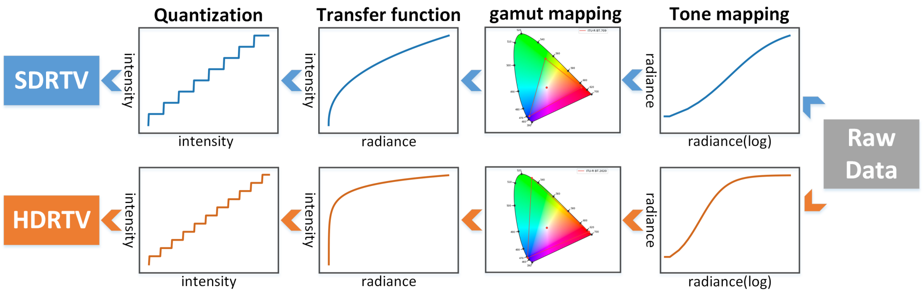

(b) SDRTV/HDRTV formation pipeline

Figure 1. (a) LDR image formation pipeline provided in SingleHDR [10]. (b) SDRTV/HDRTV formation pipeline. Raw data here does not strictly refer to Raw file, which represents content that has not been processed by the subsequent operations.

where $h(x) = ((x*(a*x+c*b)+d*e)/(x*(a*x+b)+d*f))-e/f$, and $a, b, c, d, e, f, k, w$ are specific parameters. We set $a = 0.15$, $b = 0.50$, $c = 0.10$, $d = 0.20$, $e = 0.02$, $f = 0.30$, $k = 0.2$ and $w = 11.2$. $I$ denotes radiance map. Owing to SDRTV and HDRTV have different dynamic range, we set the range of $I$ to $0-100cd/m^2$ for SDRTV and $0-10000cd/m^2$ for HDRTV. Note that we use Hable tone mapping for an example and it can actually be any tone mapping algorithm here.

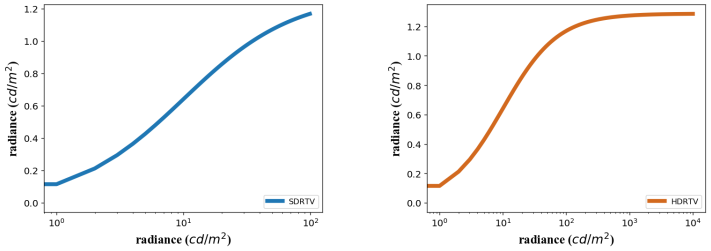

(a) (b)

Figure 2. (a) SDRTV tone mapping curve; (b) HDRTV tone mapping curve.

**Gamut mapping**. Gamut mapping is to convert colors of content from source gamut to target gamut. As shown in Fig. 3, we utilize the CIE chromaticity diagram to distinguish different target gamuts for the color gamut mapping of SDRTV and HDRTV, which correspond to rec.709 and rec.2020, respectively.

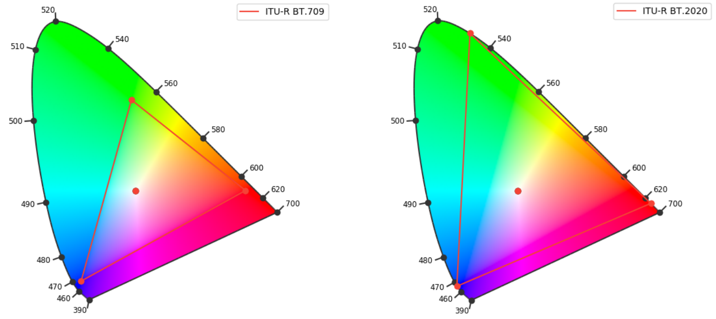

(a) (b)

Figure 3. (a) SDRTV target gamut (rec.709). (b) HDRTV target gamut (rec.2020). It can be seen that rec.2020 for HDRTV is wider than rec.709 for SDRTV in CIE chromaticity diagram

**Opto-electronic transfer function**. Opto-electronic transfer function abbreviates as OETF. It is used to convert linear optical signals to non-linear electronic signals in the image formation pipeline. We provide the gamma curve for SDRTV and PQ curve for HDRTV, as shown in Fig. 4.

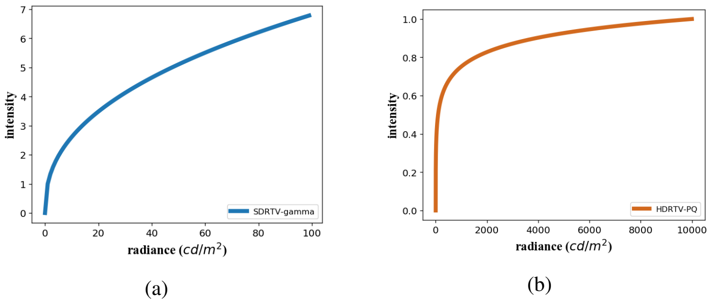


Figure 4. (a) gamma-OETF for SDRTV. (b) PQ-OETF for HDRTV.

# 3. Implementation details

For the proposed AGCM, we set the dimension of the condition vector to 6. Before training, we crop images by $480 \times 480$ with the step of 240. When training model, patches with $480 \times 480$ are input to the base network while full images downsampled by the scale of 4 are the inputs of the condition network. The mini-batch size is set to 4 and we adopt the L2 loss function and Adam [8] optimizer for training, of total $1 \times 10^6$ iterations. The initial learning rate is set to $5 \times 10^{-4}$ and decayed by a factor of 2 after every $2 \times 10^5$ iterations. For the part of LE, we use the outputs of AGCM as the inputs. The size of the mini-batch is set to 16 and the patch size is $160 \times 160$. We set the initial learning rate to $1 \times 10^{-4}$ and then decayed by a factor of 2 after every $1 \times 10^5$ iterations, of total $5 \times 10^5$ iterations. L2 loss function, Adam optimizer and Kaiming-initialization [4] are utilized for training. For training HG model, the generator is first pre-trained based on L2 loss function and Adam optimizer with a batch size of 16 and patch size of 160. The initial learning rate is set to $2 \times 10^{-4}$ and decayed by 2 after every $2 \times 10^5$ iterations, of total $5 \times 10^5$ iterations. Then, we train the GAN model with batch size of 16 and patch size of 128. The initial learning rate is set to $1 \times 10^{-4}$ and the total number of iterations is set to $4 \times 10^5$. The learning rate is decayed by a factor of 2 after every $1 \times 10^5$ iterations. Adam optimizer and Kaiming-initialization are still adopted and the L1 loss function is used for training. The weighting parameters for the losses are set to $\alpha = 0.01$, $\beta = 1$ and $\gamma = 0.005$. All models are built on the PyTorch framework and trained with NVIDIA 2080Ti GPUs.

# 4. Additional quantitative and qualitative analyses

## 4.1. Conversion from base network to 3D LUT

In many practical applications, 3D LUTs are widely used for manipulating the color and tone of images. Besides, 3D LUTs are used extensively in the movie production chain, as part of the digital intermediate process. Thus, there are many software and tools to edit images by modifying 3D LUTs. However, 3D LUTs are not flexible to interpolate and modulate as our base network for training. In previous work [11], to realize the image-adaptive function, multiple 3D LUTs are trained with a CNN weight predictor, which brings high computational cost. On the other hand, as proven in [3], a network consisting of multiple layers with only $1 \times 1$ filters can deal with many global operations well and has the flexibility to modulate the feature maps. In this part, we prove that it is easy to convert our base network to a 3D LUT with almost no loss of accuracy.

We take a 3D lattice composed of SDR colors as input and obtain a 3D LUT for SDRTV-to-HDRTV. Then, we use lookup and trilinear interpolation operations to achieve the color transformation as [11]. As in Tab. 1, 3D LUTs converted from the base network obtain comparable performance with fewer parameters. Note that the operation can also apply to our AGCM.

| Method | Params↓ | PSNR↑ | SSIM↑ | SR-SIM↑ | $\Delta E_{ITP}\downarrow$ | HDR-VDP3↑ |
|---|---|---|---|---|---|---|
| Base network | **5k** | **36.14** | **0.9643** | 0.9961 | **10.43** | 8.305 |
| 3DLUT_s33 | 108k | 35.98 | 0.9645 | 0.9988 | 10.60 | **8.322** |
| 3DLUT_s64 | 786k | 36.13 | 0.9643 | **0.9988** | 10.46 | 8.309 |

Table 1. Quantitative comparisons between base network and its converted 3D LUTs. s33 or s64 represents the size of LUT. LUTs of these two sizes are commonly used in the process of production.

## 4.2. Analysis of color mapping via LUT manifold

We provide more detailed explanations of the LUT manifold and its visualization. In the 3D LUT cube, each point has four basic attributes, which are color and three coordinate values. These three coordinate values determine the position of the color in the current domain. In Fig. 5(a), the left shows the 3D LUT cube of identity mapping. In this cube, the coordinate values of each point correspond to the three-channel values of its color in the SDR domain. We also show the LUT manifold of SDRTV-to-HDRTV color mapping using the base network in Fig. 5(b). In this cube, the coordinate values of each point represent its corresponding HDR color. We can see that SDR colors in the range of 0 to 255 are mapped to HDR colors with the range of 0 to 1023.

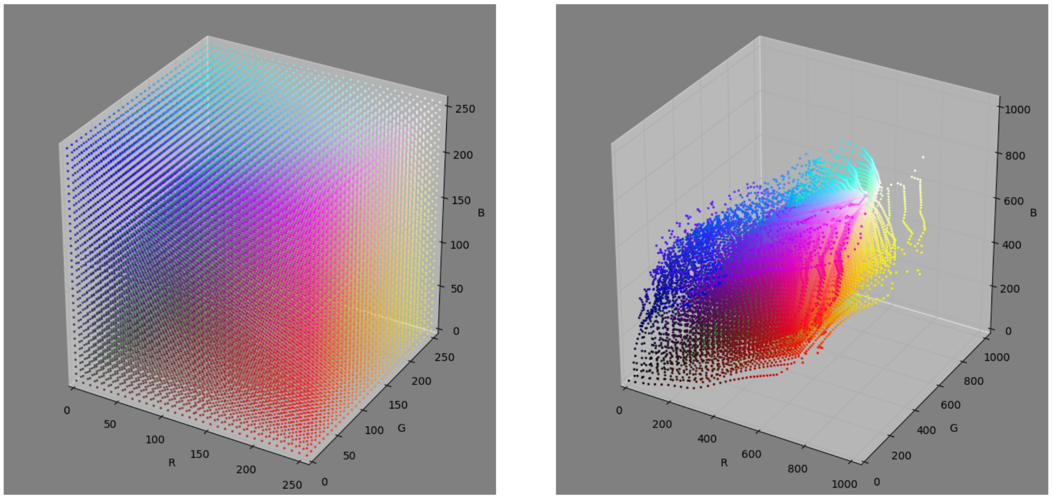


(a) Identity mapping of SDRTV colors.

(b) SDRTV-to-HDRTV color mapping of base network.

Figure 5. Visualization of 3D LUTs.

We can observe the effect of our condition network in AGCM by LUT manifold. As shown in Fig. 6, LUT manifold changes obviously by taking different images as inputs of condition network. It suggests that our AGCM achieves image-adaptive function.

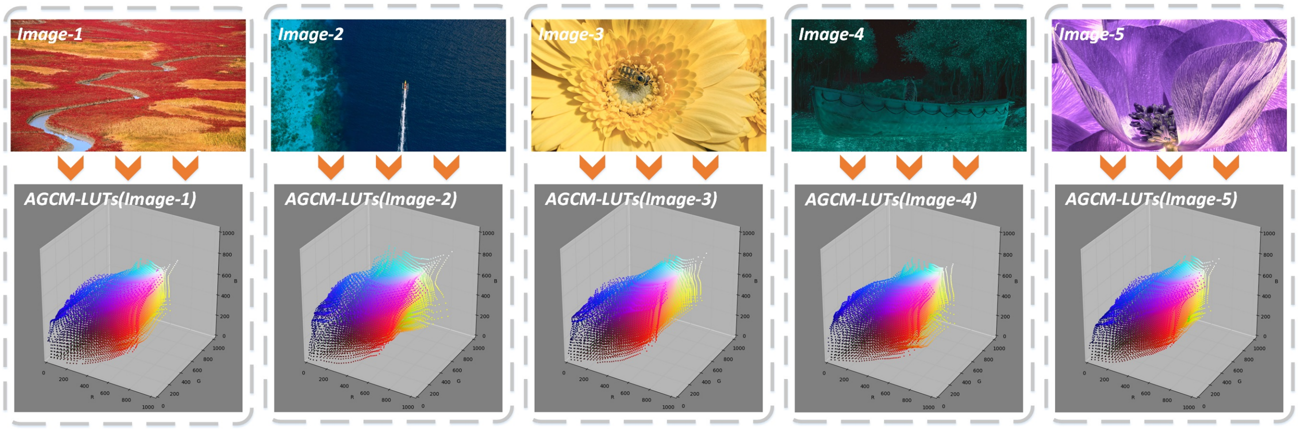


Figure 6. 3D LUTs generated by taking various images as inputs of condition network.

## 4.3. Analysis on the necessity of AGCM

We conducted some experiments to illustrate the necessity of AGCM. We make quantitative and qualitative comparisons between methods with AGCM and without AGCM. Basic3x3 represents the same network as our base network but replaces

all $1 \times 1$ filters with $3 \times 3$ filters. As shown in Tab. 2, the methods performing AGCM before LE obtain higher performance than the methods learning end-to-end mapping directly. In Fig. 7, we can see that outputs of methods without AGCM suffer obvious artifacts in some over-exposed and oversaturated regions. Besides, methods without AGCM perform badly in the color transition test. Therefore, it is necessary to perform AGCM before local enhancement. In other words, it is a better choice to perform color mapping before learning end-to-end mapping using local information.

| Method | Params↓ | PSNR↑ | SSIM↑ | SR-SIM↑ | $\Delta E_{ITP}$ ↓ | HDR-VDP3↑ |
|---|---|---|---|---|---|---|
| LE(Basic3x3) | **40K** | 36.98 | 0.9706 | **0.9989** | 9.63 | 8.368 |
| AGCM+LE(Basic3x3) | 75K | **37.50** | **0.9721** | 0.9988 | **9.13** | **8.580** |
| LE(ResNet) | **1.37M** | 37.32 | 0.9720 | 0.9950 | 9.02 | 8.391 |
| AGCM+LE(ResNet) | 1.41M | **37.61** | **0.9726** | **0.9967** | **8.89** | **8.613** |

Table 2. Quantitative comparisons between methods w/ and w/o AGCM.

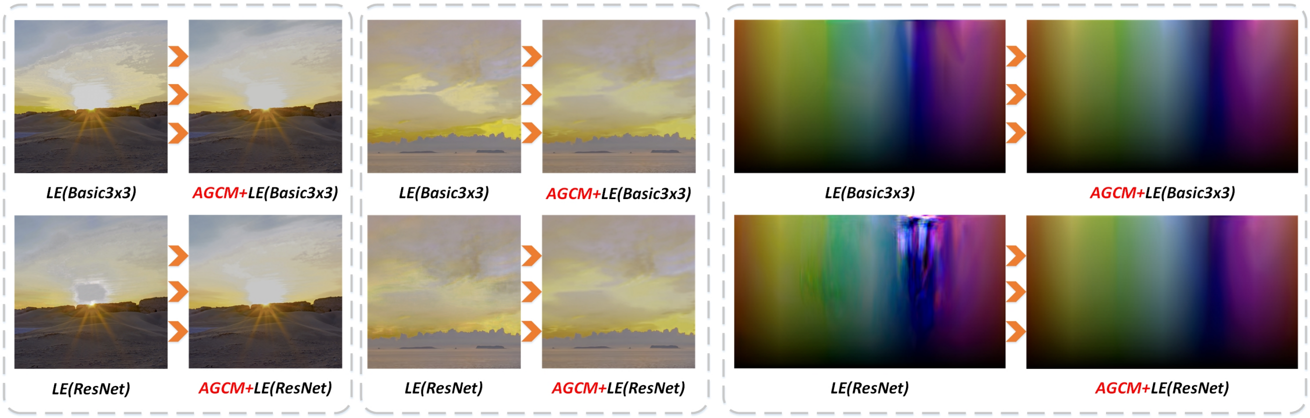


(a) Visual quality. (b) Color transition test.

Figure 7. Qualitative comparisons between methods w/ and w/o AGCM.

### 4.4. Comparisons with data-driven methods of LDR-to-HDR

As illustrated in the main paper Sec. 2 and Sec. 5.3, previous LDR-to-HDR methods are functionally different from our method. For some non-data-driven methods, we can set some variables of these algorithms to obtain considerable results for comparison. However, it is not applicable to data-driven methods, such as HDRCNN [1] and SingleHDR [10]. To illustrate this problem, we make comparisons with these two methods. In Fig. 8, the first and third columns show the outputs of these two methods processed the same as described in Sec. 5.3. Since the networks are not dedicated to the recovery of the entire range, pixel values processed by PQ-OETF are compressed to a small range. Thus, there is a lack of contrast in these results. To compare these methods as fair as possible, we manually changed the contrast of these images by multiplying the pixel value by 5. In this case, we can still observe that these methods introduce some obvious artifacts and produce

### 4.5. More comparisons with existing methods

In Fig. 10, We provide more visual comparisons of our methods against existing approaches.

## 5. Additional explanations about visualization

First of all, we must declare that the HDR results can only be displayed correctly on HDR display devices. To show the results in the paper, we visualize HDRTV images by directly showing the pixel values encoded by PQ-OETF in this work. We do this out of two considerations: (1) Displaying the PQ value directly is equivalent to linearly decoding the result. Although the images may look relatively darker than them on HDR screens, details are better preserved and can be seen more easily, especially in the highlight and saturated regions. (2) Visualized results by tone mapping as [6, 7] are closer to the intuitive feeling of HDR, but the artifacts, which can be easily seen on HDR display devices, may be reduced and not easily visible in paper, as shown in Fig. 11.

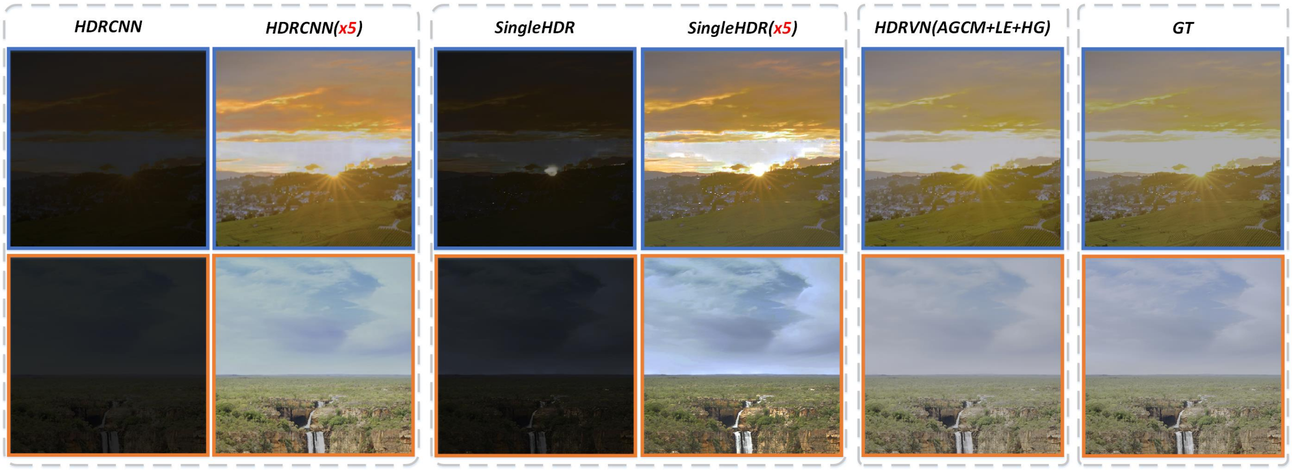


Figure 8. Qualitative comparisons. The top row describes the categories of algorithms.

## 6. Additional explanations about the user study

In this section, we provide more explanations about how we conduct the user study. As described in the main paper Sec. 5.6, we randomly select 25 images from the testing set and show results of the images produced by different methods to participants on HDR-TV in dark conditions. The HDR-TV is Sony X9500G with a peak brightness of 1300 $cd/m^2$. Before experimenting, we first instruct the participants to take the following three factors as the main evaluation considerations: (1) whether there are obvious artifacts and unnatural colors, (2) whether the overall color, brightness and contrast of the images are natural and comfortable, (3) whether the contrast between light and dark levels and highlight details can be perceived. Based on these three principles, participants are asked to rank the results of different methods in each scenario. When displaying the results, the TV is set to rec.2020 color gamut and HDR10 standard. We compared five methods including Ada-3DLUT [11], Deep SR-ITM [6], Pixel2pixel [5], KovaleskiEO [9] and our method with Ground Truth. When ranking the images for a certain scene, participants can observe six images of different methods at the same time or compare any two pictures at will until they decide the order. We show the counts of different results in the top three ranks, as shown in the main paper Fig. 6. There are 208 (41.6%) and 86 counts (17.2%) for GT and our method, respectively. It means that among the results considered to have the best visual quality, GT and our method account for 41.6% and 17.2%, respectively. Similarly, the results of our method account for 35.4% among the results considered to be the second-best visual quality. In conclusion, the results obtained by our method are second only inferior to GT in terms of visual quality.

## 7. Realistic SDRTV-to-HDRTV

We test our HDRTVNet on native 4K videos to demonstrate the performance of conversion in realistic scenes. To revive landscape viewing as far as possible, we employ an HDR camera* fixed by a tripod to shot the same frame of HDRTV/SDRTV respectively and directly show the JPG images processed by the camera. In Fig. 9, we can observe that the generated results have more vivid color and higher contrast than their SDRTV versions.

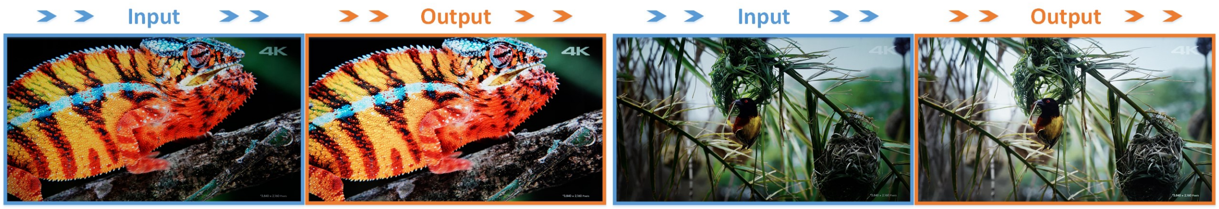


Figure 9. Predictions for realistic conditions.

*The camera we use is Sony ILCE-7M2, whose light measuring range is EV-1∼EV20.

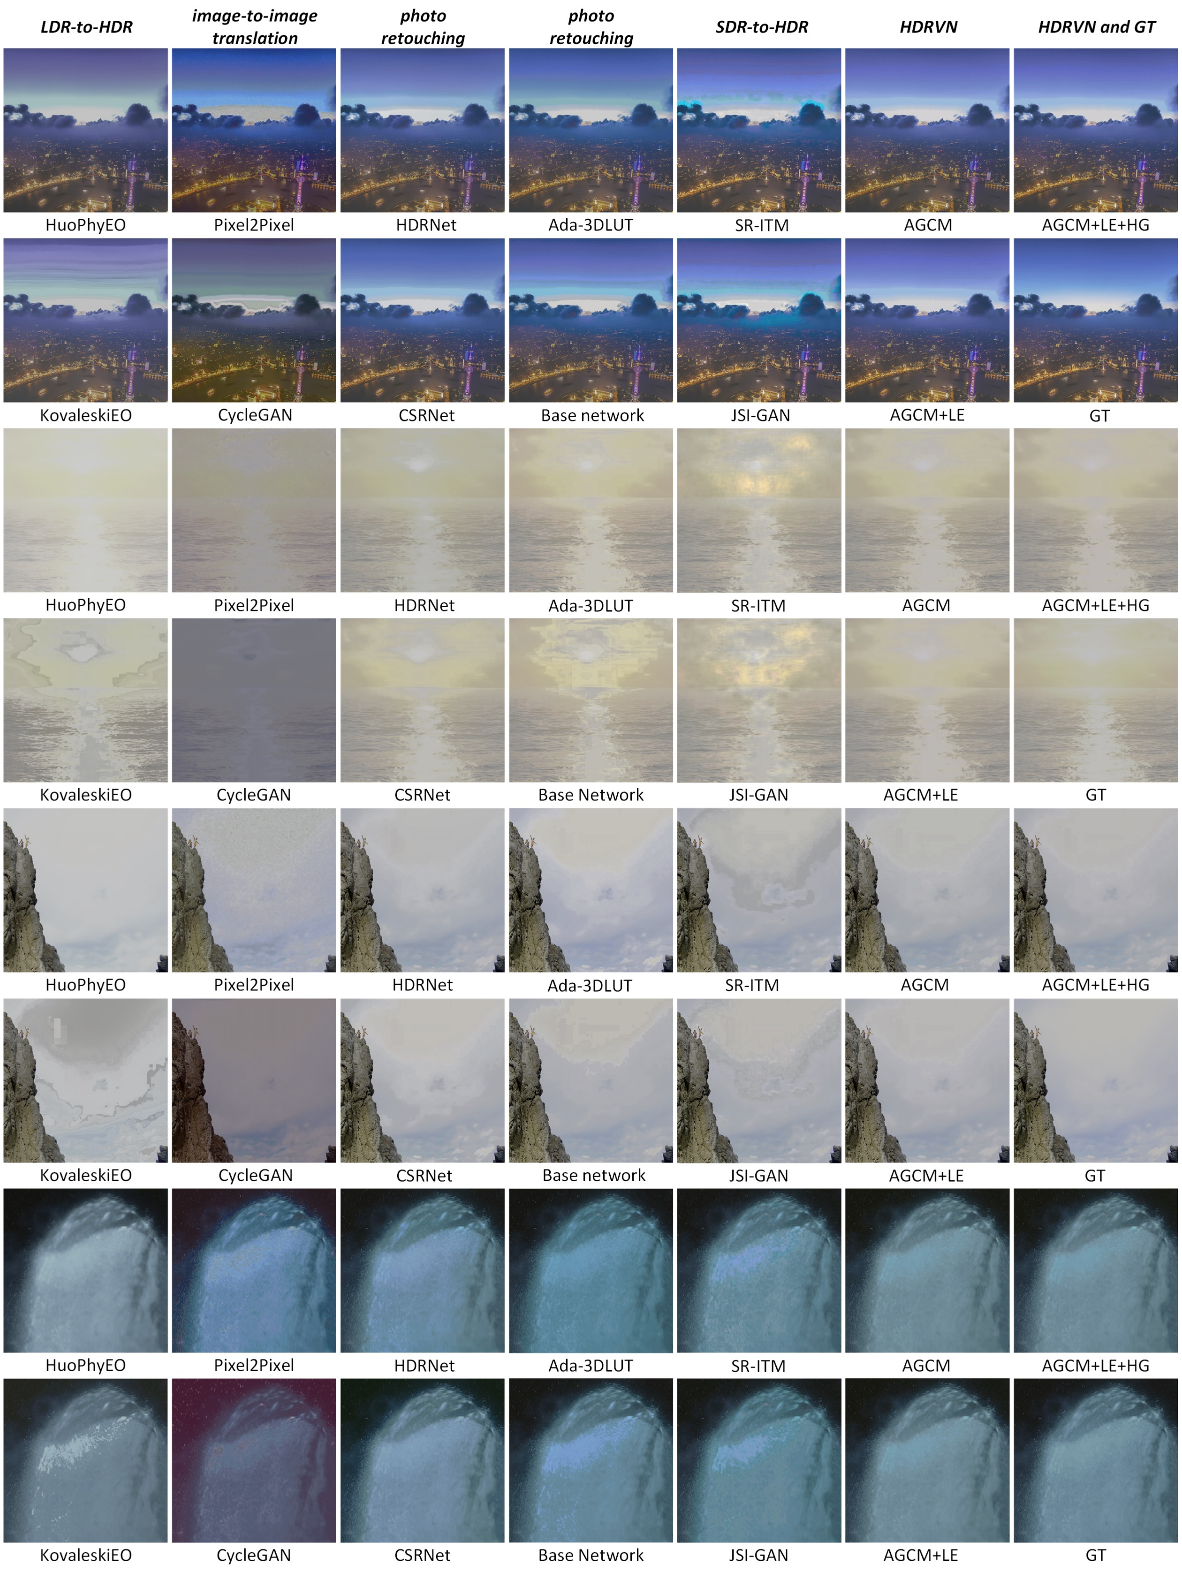


Figure 10. Qualitative comparisons. The top row describes the categories of algorithms.

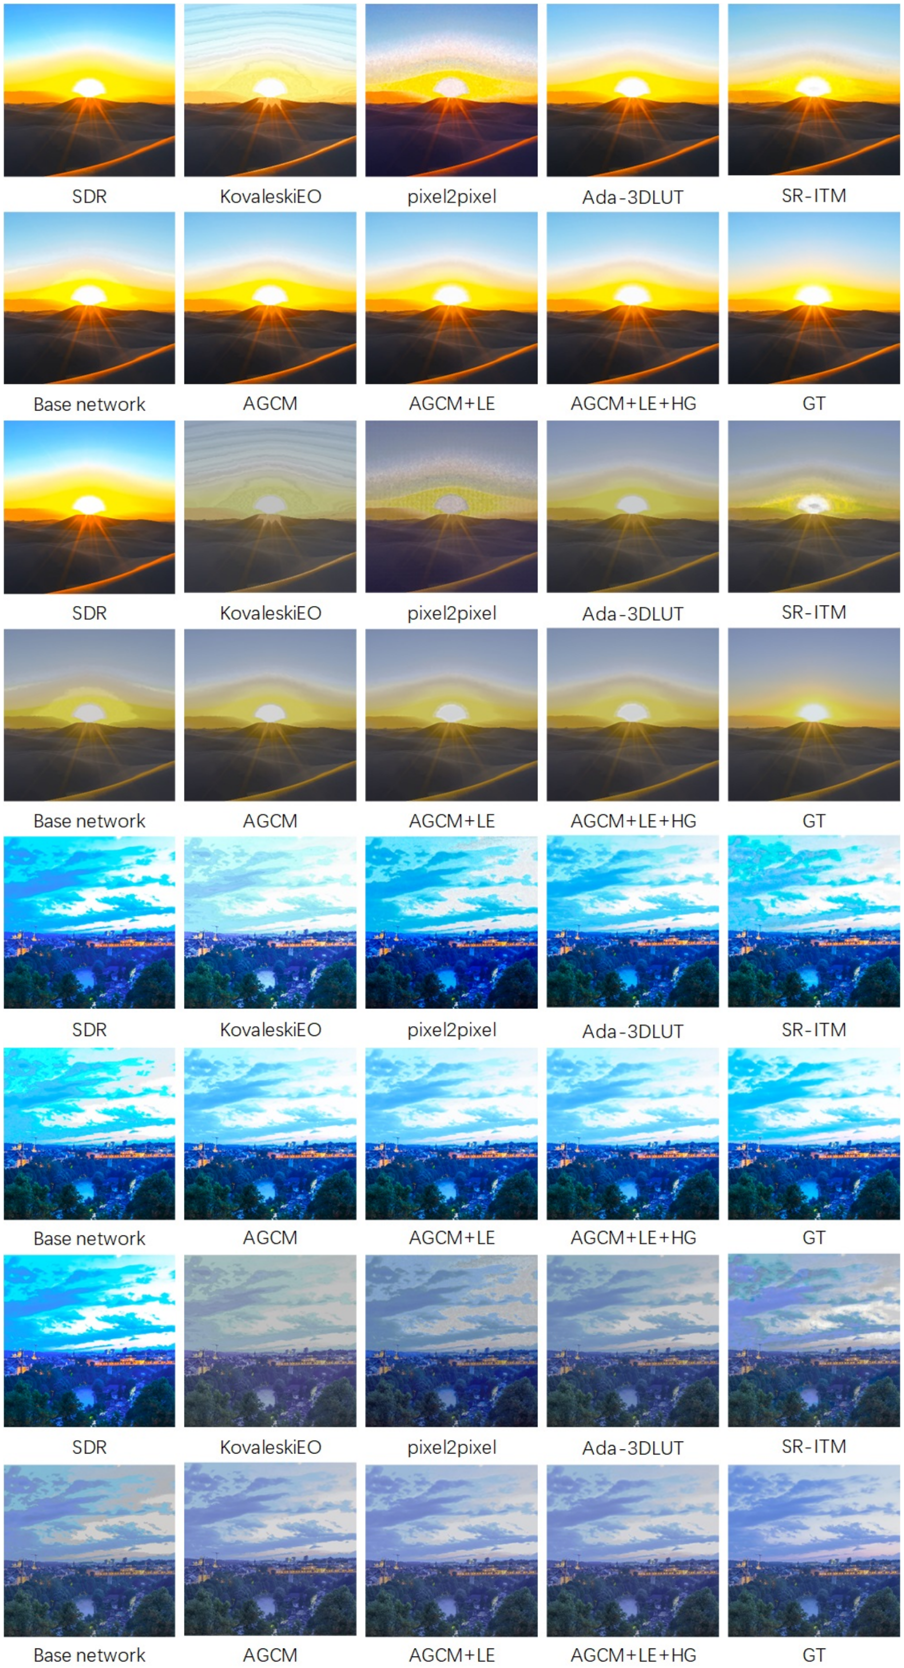


Figure 11. Comparison of visualization methods. The first two rows of every four rows are tone mapped results.

## References


[1] Gabriel Eilertsen, Joel Kronander, Gyorgy Denes, Rafał K Mantiuk, and Jonas Unger. Hdr image reconstruction from a single exposure using deep cnns. *ACM transactions on graphics (TOG)*, 36(6):1–15, 2017. 5

[2] John Hable. Uncharted 2: Hdr lighting. In *Game Developers Conference*, page 56, 2010. 1

[3] Jingwen He, Yihao Liu, Yu Qiao, and Chao Dong. Conditional sequential modulation for efficient global image retouching. *arXiv preprint arXiv:2009.10390*, 2020. 3

[4] Kaiming He, Xiangyu Zhang, Shaoqing Ren, and Jian Sun. Delving deep into rectifiers: Surpassing human-level performance on imagenet classification. In *Proceedings of the IEEE international conference on computer vision*, pages 1026–1034, 2015. 3

[5] Phillip Isola, Jun-Yan Zhu, Tinghui Zhou, and Alexei A Efros. Image-to-image translation with conditional adversarial networks. In *Proceedings of the IEEE conference on computer vision and pattern recognition*, pages 1125–1134, 2017. 6

[6] Soo Ye Kim, Jihyong Oh, and Munchurl Kim. Deep sr-itm: Joint learning of super-resolution and inverse tone-mapping for 4k uhd hdr applications. In *Proceedings of the IEEE International Conference on Computer Vision*, pages 3116–3125, 2019. 5, 6

[7] Soo Ye Kim, Jihyong Oh, and Munchurl Kim. Jsi-gan: Gan-based joint super-resolution and inverse tone-mapping with pixel-wise task-specific filters for uhd hdr video. In *AAAI*, pages 11287–11295, 2020. 5

[8] Diederik P Kingma and Jimmy Ba. Adam: A method for stochastic optimization. *arXiv preprint arXiv:1412.6980*, 2014. 3

[9] Rafael P Kovaleski and Manuel M Oliveira. High-quality reverse tone mapping for a wide range of exposures. In *2014 27th SIBGRAPI Conference on Graphics, Patterns and Images*, pages 49–56. IEEE, 2014. 6

[10] Yu-Lun Liu, Wei-Sheng Lai, Yu-Sheng Chen, Yi-Lung Kao, Ming-Hsuan Yang, Yung-Yu Chuang, and Jia-Bin Huang. Single-image hdr reconstruction by learning to reverse the camera pipeline. In *Proceedings of the IEEE/CVF Conference on Computer Vision and Pattern Recognition*, pages 1651–1660, 2020. 1, 2, 5

[11] Hui Zeng, Jianrui Cai, Lida Li, Zisheng Cao, and Lei Zhang. Learning image-adaptive 3d lookup tables for high performance photo enhancement in real-time. *IEEE Transactions on Pattern Analysis and Machine Intelligence*, 2020. 3, 6
